# Supplementary material for: Qubits, entangled states, and quantum gates realized on a set of classical pendulums
Source: arXiv:2312.00631 source file (2023-12-01)
Supplement: Supplementary file 1 [file qubits_supplementary.pdf]

# Supplementary Materials:
# Qubits, entangled states, and quantum gates realized on a set of classical pendulums

Alexey V. Nenashev,[1] Florian Gebhard,[1] Klaus Meerholz,[2] Sergei D. Baranovskii[1,2]

[1] Department of Physics and Material Sciences Center, Philipps-University, D-35032 Marburg, Germany,
[2] Department für Chemie, Universität zu Köln, Luxemburger Strasse 116, 50939 Köln, Germany

## S1. Berry phase and Foucault pendulum

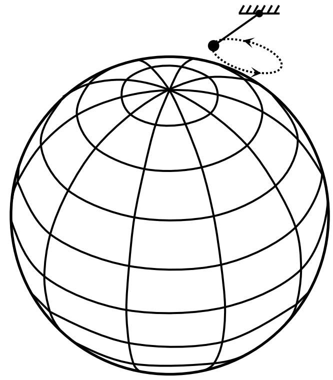

So far, we depicted a system with two degrees of freedom as two pendulums moving in a plane. Here we use another possible representation — as one pendulum in three-dimensional space, which is allowed to move along two coordinates. Let this pendulum be immersed in the gravitational field of some planet. For simplicity, we assume that the planet does not rotate, although we are going to draw a grid of parallels and meridians on it.

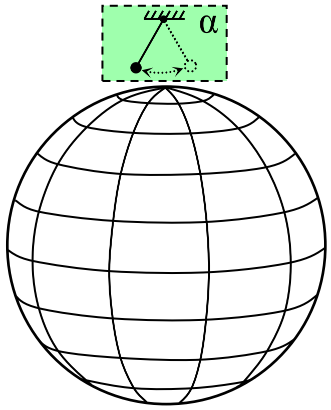


Suppose that the pendulum is initially placed at the pole of the planet, and swings in some plane α.

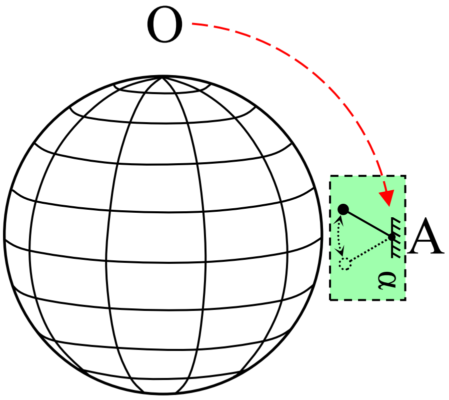


Let us slowly move the point where the pendulum is suspended (the pivot) from the pole (point O) to the equator (point A) along the meridian lying in the same plane α. Since all the forces acting on the pendulum are parallel to the same plane, the pendulum continues to oscillate in the plane α.

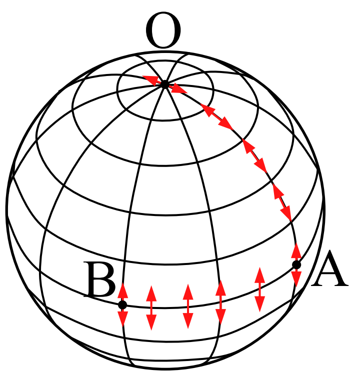


At the point A, the pendulum oscillates across the equator. Now let's slowly move the pendulum along the equator from point A to some point B. One can conclude from symmetry considerations that during this movement the pendulum will oscillate perpendicular to the equator all the way. (The double arrows on the figure show the plane of the pendulum oscillations when its suspension point moves.)

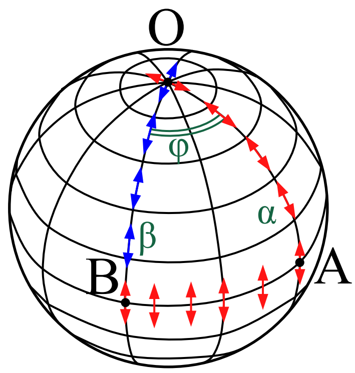


At the point B, the pendulum oscillates in some plane β passing through the suspension point and the poles of the planet. Let us now return the suspension point to the pole, moving it along the meridian lying in the plane β. The same arguments as those above lead to the conclusion that the oscillations of the pendulum will remain in plane β.

Because of this “journey”, the plane of the pendulum oscillations has turned by a certain angle φ, namely, the angle between the planes α and β. This angle is equal to the area of the spherical triangle OAB on the surface of the planet divided by the square of the planet radius.

Note that the angle of rotation φ does not depend on the speed with which the pendulum is moved around the planet, but depends only on the trajectory of the movement. This is true, however, only for a slow (adiabatic) movement, the characteristic time of which is large compared to the period of pendulum oscillations.

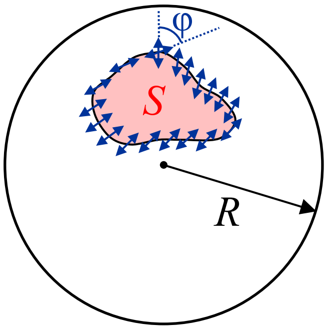


This result is easily generalized to the case when we carry the pendulum on the planet along an arbitrary closed path. Namely, the plane of pendulum's oscillations at the end of the path is rotated by some angle φ compared to the plane of oscillations at the beginning. This angle φ does not depend on how fast we move the pendulum, as long as we do it adiabatically slowly. The angle φ is proportional to the area *S*, which is “cutted out” from the planet’s surface by the path of the pendulum:

$$\varphi = S / R^2,$$

where *R* is the planet’s radius. One can prove this formula by breaking the area *S* into small triangles and using the fact that the sum of angles of a triangle on a sphere is $2\pi + S_\Delta/R^2$, where $S_\Delta$ is the triangle’s area.

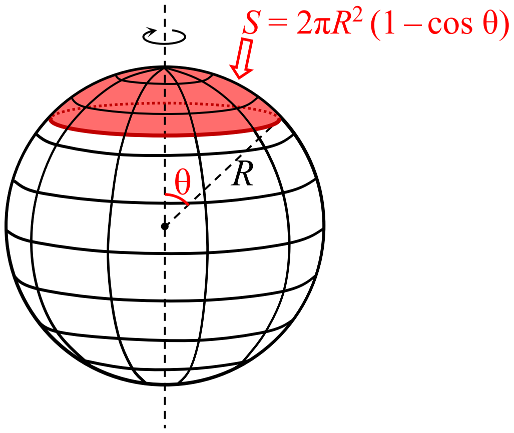


An important example is when the pendulum is fixed on the planet, but the planet itself rotates around its axis. From the point of view of a stationary observer, the suspension point moves in a circle along some parallel. The area *S* to the north of the parallel is equal to

$$S = 2\pi R^2 (1 - \cos\theta) = 2\pi R^2 (1 - \sin\chi),$$

where θ is the polar angle, and $\chi = (\pi - \theta)$ is the latitude. From the point of view of a stationary observer, the plane of the pendulum turns by an angle $\varphi = S / R^2 = 2\pi\,(1 - \sin\chi)$ during one period *T* of the planet rotation. From the point of view of an observer that rotates with the planet, the turning angle of the pendulum oscillation plane is $\tilde{\varphi} = \varphi - 2\pi = -2\pi\sin\chi$ per one period *T*. Hence, looking from the reference frame that rotates with the planet, one can see that the plane of pendulum’s oscillations rotates with angular frequency

$$\tilde{\varphi}/T = -(2\pi/T)\sin\chi = -\Omega\sin\chi,$$

where Ω is the angular frequency of the planet. The same result can be obtained in the usual way — by considering the action of the Coriolis force on the pendulum. Such a pendulum,

the plane of oscillation of which rotates due to the rotation of the planet, is called a **Foucault pendulum**.

The angle of rotation φ does not depend on the plane, in which we initially swung the pendulum. We can generalize this statement and say that whatever the initial movement of the pendulum weight (back-and-forth, elliptical, or circular), after transferring its suspension point along a closed trajectory, the pendulum will come to the same state of motion but rotated by an angle $\varphi = S / R^2$. For example, if the initial movement of the weight was circular, then it remains circular when the pendulum completes its "journey" on the surface of the planet, while the phase of this movement will receive an increment $\varphi = S / R^2$.

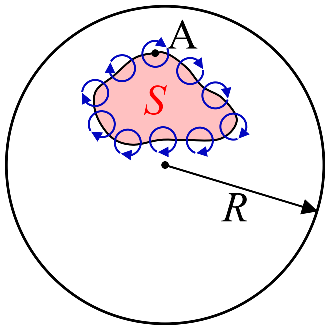


To support this conclusion, let us imagine that we have two pendulums, a red one and a blue one, which were initially put into the same circular motion, i.e., their weights moved synchronously. The blue pendulum is always at the same point A of the planet, and the red one was moved from point A along a closed path on the surface of the planet, and eventually returned to the same point A.

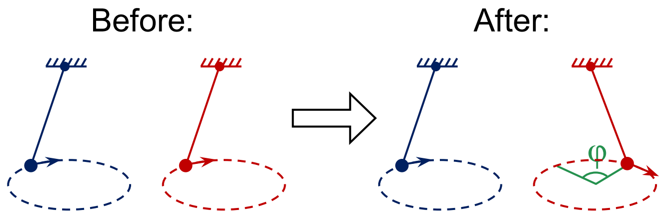


Looking at the position of weights after an integer number of their periods of oscillation, one can see the blue pendulum in exactly the same state of motion. Notably, the red pendulum has turned by an angle φ in comparison with the blue one, and thus "overtook" it in phase by φ. If the pendulums were launched in the opposite direction, counterclockwise, then the red pendulum, on the contrary, would be behind the blue one in phase by φ.

Let us now translate this observation from the "language of pendulums" into the language of quantum theory. Two degrees of freedom of the pendulum's motion correspond to a two-level quantum system. In the pendulum transfer experiment, however, the states of the clockwise and counterclockwise circular motions "do not mix". Therefore, one can leave in consideration only one quantum level, which corresponds to the circular movement of the pendulum weight in a clockwise direction.

The equation of motion of a pendulum depends on the position of its suspension point on the planet, i.e., on the latitude and the longitude. Translated into "quantum language" this means that the Hamiltonian of the corresponding quantum system depends on two continuous parameters, the latitude and the longitude. When the pendulum is moved along a closed trajectory on a surface of the planet, this means in "quantum language" that the Hamiltonian smoothly changes in a two-dimensional space of the latitude-longitude parameters. If this is done adiabatically slowly and ends up at the same point A in the parameter space, from which we started, then the quantum system (with one isolated level) will also return to its original state. However, this state will acquire an additional phase factor $e^{i\varphi}$ in comparison with the "control experiment", in which the Hamiltonian did not change. The phase shift φ is called the **geometric phase**, or the **Berry phase**.

The Berry phase is an important concept in modern quantum theory. For example, it plays a significant role for understanding the properties of topological insulators.

The value of the Berry phase φ does not depend on the speed of movement in the parameter space (i. e., on the speed of changing the Hamiltonian). It depends only on the trajectory in the parameter space, i. e., on the continuous sequence of Hamiltonians.

In the above example with the pendulum and the planet, the Berry phase is proportional to the area $S$ inside the trajectory on the planet's surface. In the general case, when the Hamiltonian depends on two arbitrary parameters $P_1$ and $P_2$, the Berry phase is given by the area integral inside the trajectory: $\varphi = \int K(P_1, P_2)\, dS$, where function $K(P_1, P_2)$ is called the **Berry curvature**. In our example, the Berry curvature is constant and equal to the Gaussian curvature of the planet's surface: $K(P_1, P_2) = 1 / R^2$. When the parameter space is three-dimensional, then the Berry curvature is a vector quantity. The Berry phase is then equal to the flow of this vector through a closed trajectory of motion in the parameter space.

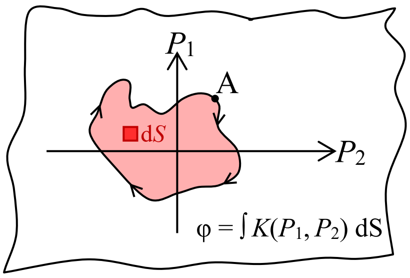


## S2. Why quantum error correction is necessary

Consider three light switches hanging on the wall, while an earthquake (not catastrophic) occurred. What has happened to the switches? Nothing: those, which were switched on remain switched on, and those, which were switched off remain off. This is an example of the fact that bits of ordinary classical information are resistant to physical perturbations.

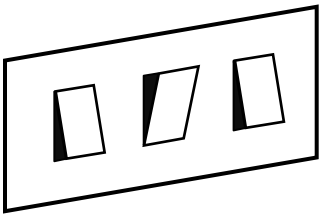

Let us now consider eight swinging pendulums, which model three qubits, as illustrated in Fig. 5a., while an earthquake occurred. Could we hope that the state of pendulums' motion did not change during the earthquake? Not at all.

This is one of the main differences between classical and quantum information: the latter is subjected to external perturbations, even if these perturbations are arbitrarily weak. To understand this difference better, recall that a switch contains a very important detail — a latch fixed by a spring. This latch protects the switch from changing its state under the (not very strong) perturbations. In the language of dynamical systems, a latch is a nonlinear dissipative element. In computer memory, the role of such nonlinear elements is played by transistors. However, we cannot "attach" any nonlinear dissipative element to our pendulums. It is because the pendulums are served to mimic the evolution of a quantum system, and the latter is governed by *linear* unitary transformations.

How then, under these circumstances, to protect quantum information from external influences? If the influence is arbitrary (i. e., described by a general Hamiltonian), then protection seems to be impossible. However, one can protect quantum information against certain types of influence. For this purpose, the methods of quantum error correction have been invented.

Let us illustrate the idea of a quantum error correction on the simplest example, when the error occurred by flipping a qubit (NOT gate) with a certain probability. We will assume this probability small, so we will neglect the events of the flip of two (or more) qubits at the same time. Suppose a qubit in some unknown state $\alpha\,|\downarrow\rangle + \beta\,|\uparrow\rangle$ that should be protected from the flip events. Let us add two auxiliary qubits (ancillas) to the system, and encode the state under protection in three qubits as follows: $\alpha\,|\downarrow\downarrow\downarrow\rangle + \beta\,|\uparrow\uparrow\uparrow\rangle$. One **logical qubit** is, therefore, encoded in three **physical qubits**. In the pendulum model, it looks like

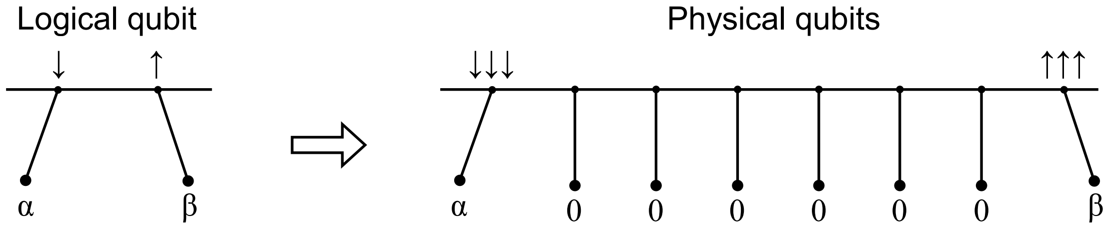


(Here, the complex amplitudes of oscillations, α, β, or zeros are ascribed to each pendulum.) This is an entangled state of three physical qubits.

Then four options for flips of a qubit are possible: (0) no flips, (1) the 1st qubit has flipped, (2) the 2nd qubit has flipped, or (3) the 3rd qubit has flipped. Let us depict the state of motion of the pendulums in each of these options:

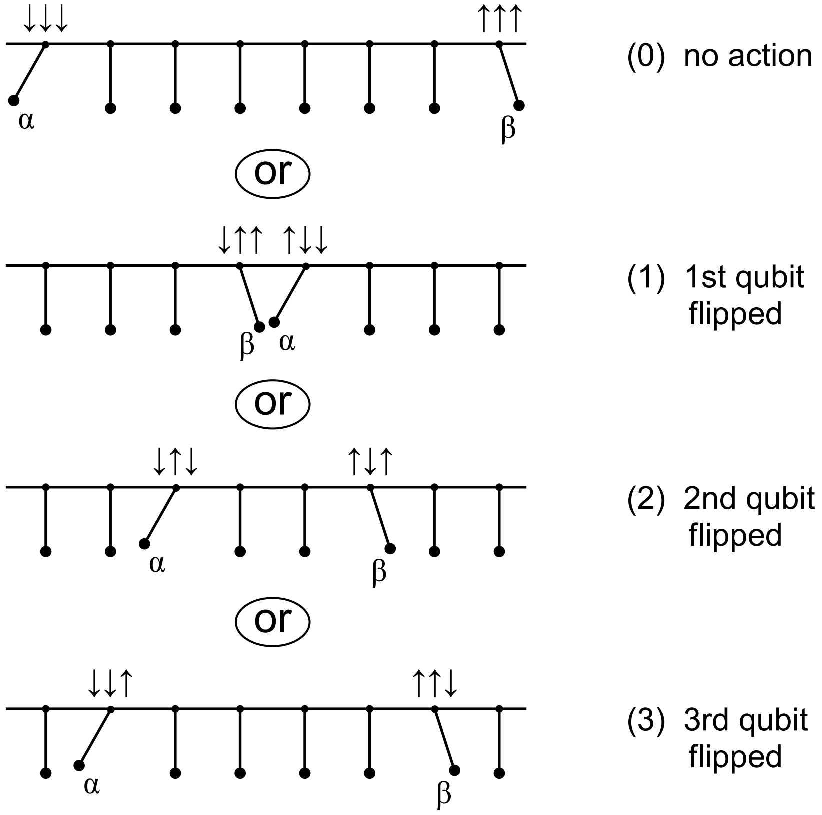


Let us now rearrange the pendulums in the following order: 1st, 8th, 5th, 4th, 3rd, 6th, 2nd, 7th. This can be done using a suitable sequence of quantum gates. The pendulum motions after this permutation will be the following ones:

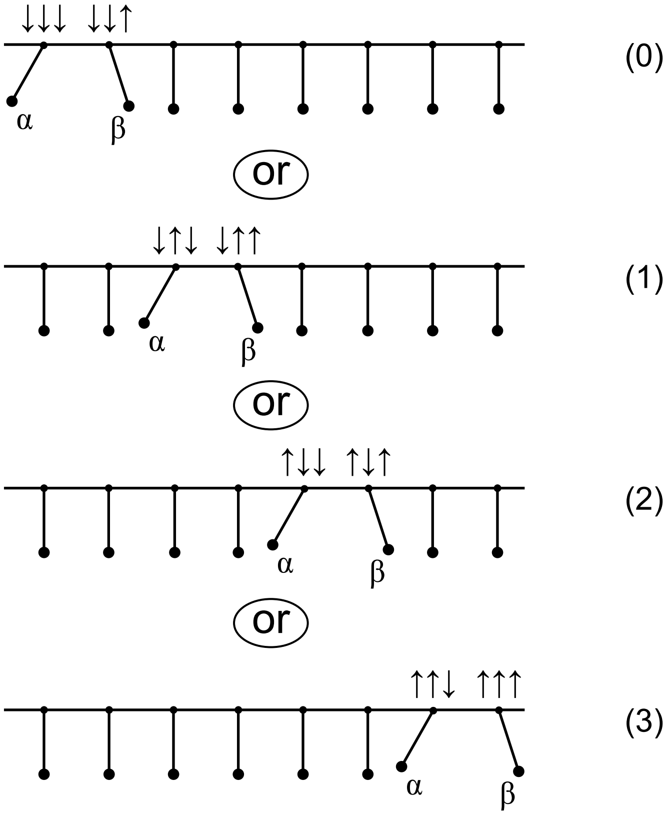


These states can be rewritten in the quantum language as follows:

$|\downarrow\rangle\, |\downarrow\rangle\, (\alpha\, |\downarrow\rangle + \beta\, |\uparrow\rangle)$ in case (0),
$|\downarrow\rangle\, |\uparrow\rangle\, (\alpha\, |\downarrow\rangle + \beta\, |\uparrow\rangle)$ in case (1),
$|\uparrow\rangle\, |\downarrow\rangle\, (\alpha\, |\downarrow\rangle + \beta\, |\uparrow\rangle)$ in case (2),
$|\uparrow\rangle\, |\uparrow\rangle\, (\alpha\, |\downarrow\rangle + \beta\, |\uparrow\rangle)$ in case (3).

It is clearly seen that, in each case, the state of the 3rd qubit is equal $\alpha\, |\downarrow\rangle + \beta\, |\uparrow\rangle$, i. e. to the initial state of the logical qubit. In other words, the initial state of the logical qubit has been preserved in the state of the 3rd qubit.

States of the 1st and 2nd qubits, on the contrary, are determined on whether some qubit was flipped. It is said that these qubits store the error syndrome. We do not need it anymore, so that the 1st and 2nd qubits can be initialized (that means erasing of information) and reused.

This example shows that one logical qubit encrypted in three physical qubits can be protected from flipping any of these physical qubits. In reality, the set of possible errors is much wider than just flips of qubits. For this reason, the quantum error correction protocols require a huge number (hundreds) of physical qubits per one logical qubit. When (and if) the experimental facilities allow such a large number of qubits with a sufficiently low error probability, then it will be possible to perform the so-called fault-tolerant quantum computations, in which quantum information will be protected from external influences.
